# Supplementary material for: SDAT: Sub-Dataset Alternation Training for Improved Image Demosaicing
Source: arXiv:2303.15792 source file (2024-02-12)
Supplement: Supplementary file 1 [file supplementary.tex]

\newpage
\label{sec:supplementary}
  
    
   

% \newfloat{algorithm}{htbp}{loa}[figure]
% \floatname{algorithm}{Algorithm}
% \renewcommand{\thealgorithm}{S\arabic{algorithm}}
\section{Method}
\subsection{Sub-datasets identification and creation}
In the following we provide a more detailed explanation for the sub-datasets generation process.\\
{\bf Generation of Sub-datasets}:
As an initial step we train a base model on the entire dataset. We denote the initial predicted patch $\hat{P}_{init}$ and the patch in the ground-truth RGB image as $P$, both of size $H_p \times W_p \times 3$. Then, we collect different types of patches by using a variety of metrics and create a pool of sub-datasets.
Each sub-dataset consists of the 5 percent patch subset which produces the largest metric error. The following custom metrics are used for this stage:
\begin{enumerate}
    \item \textit{Zipper metric} - this metric $d_{zip}$ is used to find zipper artifacts near edges in the image. First we calculate a mask $M_{NE}$ to identify non-edge areas as follows
    \begin{equation}
        \label{eq:MNE}
        M_{NE} := | C( \hat{P}_{init} ) - C\left( P \right) | < \varepsilon_1,
    \end{equation}
    where $C$ is some kind of edge detector, \eg Canny, and $\varepsilon_1$ is a predefined threshold.
    Then we are able to calculate
    \begin{equation}
        \label{eq:HZ}
        d_{zip} := \| | \, | \nabla \hat{P}_{init} | - \left| \nabla P \right| |  \odot M_{NE} \|_1,
    \end{equation}
    where $ \left| \nabla \right| = \left|\frac{\partial}{\partial x} \right| + \left|\frac{\partial}{\partial y} \right|$, and $\odot$ is the element-wise product.
    
    \item \textit{Grid metric} - this metric $d_{grid}$ is used to find grid-like artifacts in flat areas as follows
    \begin{multline}
        \label{eq:HG}
        d_{grid} := \| 2 \cdot | \nabla \hat{P}_{init} | \, \odot \\
        ( \sigma ( \frac{\alpha}{\left| \nabla P \right|}  ) -0.5 ) \odot ( | \nabla \hat{P}_{init} | > \varepsilon_2 ) \|_1,
    \end{multline}
    where $\sigma$ is the Sigmoid function, $\alpha > 0$ is a parameter that scales the values of the Sigmoid, and $\varepsilon_2$ is another predefined threshold.

    \item $L_1$ \textit{distance} - a simple photometric distance.
    \begin{equation}
    \label{eq:L1}
        d_{L_1}: = \| \hat{P}_{init} -  P  \|_1     
    \end{equation}

    \item \textit{Perceptual metric} \cite{ledig2017photo} - this metric $ d_{VGG/i.j} $ is used for capturing the perceptual distance between the source and predicted patches.
    \begin{equation}
	\label{eq:vgg}
	    d_{VGG/i.j} := \| \phi_{i,j}(\hat{P}_{init}) - \phi_{i,j}(P) \|^2_2,
	\end{equation}
    where $\phi_{i,j}$ indicates the feature map obtained by the j-th convolution (after activation) before the i-th maxpooling layer within the pre-trained VGG19 network \cite{simonyan2014very}.
    
    \item \textit{Edge distance} - This metric $d_{edge}$ is used to find distortions around edges
    \begin{equation}
	\label{eq:edge}
	    d_{edge} := \| C( \hat{P}_{init} ) - C\left( P \right) \|_1.
	\end{equation}
    
\end{enumerate}

Note, some sub-datasets are generated by changing the threshold of the metric such as in \Cref{eq:HG}. \\
\subsection{Selection and elimination of sub-datasets}
Our method for selecting sub-datasets is presented in the pseudo code \Cref{alg:IdentifyingDesiredDataCategories}. We outline the method for selecting specific sub-datasets among the collected pool of sub-datasets. The method involves two steps: In step 1 we re-train the base model that was previously trained on the entire dataset. The re-training is performed on one of the sub-datasets. We calculate the validation loss curves on all the sub-datasets, as well as the validation loss curve over the entire dataset. We then check if the validation loss curve on the trained sub-dataset is negatively correlated with the validation loss curve on the entire dataset. If so, the sub-dataset is added to a dictionary called "category bank". In step 2, the algorithm checks the correlation between the validation loss curves for each pair of sub-datasets in the bank. If the correlation is positive, the algorithm combines the two sub-datasets into a single sub-dataset. We use Spearman's rank correlation coefficient to measure the correlation between the validation loss curves. The algorithm also includes a threshold parameter ($Th_1$) to determine when a correlation is considered significant and another threshold parameter ($Th_2$) to determine when two sub-datasets should be merged.

% Pseudo code  \Cref{alg:IdentifyingDesiredDataCategories}. This pseudo code outlines the method for selecting specific sub-categories among the mined sub-categories. The method involves two steps: In step 1, we use a pre-trained model to train each mined sub-category and calculate its validation loss curve, as well as that of the original dataset. We then check if the validation loss curve for a given sub-category is negatively correlated with the validation loss curve for the original dataset. If so, the sub-category is added to a dictionary called "bank categories". In step 2, the algorithm checks the correlation between the validation loss curves for each pair of sub-categories in the bank. If the correlation is positive, the algorithm combines the two sub-categories into a single sub-category.

\begin{algorithm}
\small 
\caption{Identifying Sub-DataSets}
\label{alg:IdentifyingDesiredDataCategories}
\SetAlgoLined
\DontPrintSemicolon 

% \textbf{Input}: Pre-trained model trained on all dataset, mined data categories.

% \textbf{Output}: Non correlate data categories.

\KwIn{ \textbf{generalModel} as pre-trained model trained on general dataset \\ \textbf{allSubCategories} as the mined sub-categories}
\KwOut{Non correlated sub-categories}

\medskip
 
\textbf{Step 1. Inverse-correlation:} \\ 
     allValiCurves = $\{ \}$, CateogryBank = $\{ \}$ \\ 

    \For{ subCategory  {\normalfont in} allSubCategories}
        {   
        \begin{enumerate}
            \item Load \textit{generalModel} into  \textit{model}
            \item Train \textit{model} on \textit{subCategory}
            \item Calculate the validation loss curve for all mined categories, including general dataset validation curve.
            \item \textit{valiCorr} $\gets$ \textbf{corr}(\textit{genlVali}, \textit{SubCatVali})
            \item     \If{  valiCorr $< Th_1 $   }
            { 
                \tcp*{Negative correlation response}
                \hspace{3mm} CateogryBank $\gets$ sub category; \\
                \hspace{3mm} allValiCurves[subCategory]  $ \gets $ all categories validation errors
            }
        \end{enumerate} }
        
   allValiCurves output:
    \begin{tabular}{l l}
    Sub-category1: & all validation curves \footnotesize (trained on \\ sub-category1)\\ 
        ... & ... \\
    Sub-categoryN: & all validation curves \footnotesize (trained on \\ sub-categoryN) \\ 
    \end{tabular} \\ ~ \\ 

\textbf{Step2. Inter-correlation between sub-categories:}
 
\For{subCategory  {\normalfont in}  CategoryBank}
    {
    \begin{enumerate}
        \item  \textit{valiCurvesSubCategory} $\gets$  \textit{allValiCurves}[\textit{subCategory}] 
        % \item  ValSubCategory - validation curve for sub-category trained over sub-category.  
        % \item Get all validation curves over all categories during\\the training over sub-category. 'ValidationCategories[\textbf{SubCategory}]'

        \item  \textit{selfValiCurv} $\gets$  \textit{ValiCurvesSubCategory}[\textit{subCatagorey}]
        
       \item \For{otherValiCurv {\normalfont in} valiCurvesSubCategory}
        {
            \vspace{1mm}  \textit{valiCorr} $\gets$ \textbf{corr}( \textit{selfValiCurv},  \textit{otherValiCurv})
            
            \If{  valiCorr $> Th_2 $ \\ }
            {
               \hspace{-5mm} \tcp*{Positive correlation response}
                
                \textbf{merge}  \textit{otherCategory} with  \textit{subCategory} in \textit{CategoryBank}
            }
        }
    \end{enumerate} 
    } 
  \textbf{Return}  CategoryBank.
\end{algorithm}

\section{Experiments}
\subsection{SDAT method settings:}
\textbf{Learning rate scheduler:}
Every training phase on a chosen sub-dataset the LR is initialized to $\frac{Base ~ LR}{10}$ and increases till the end of the phase to $10 \times Base ~ LR$. See \cref{S:LR_SCHEDULER}.
\begin{figure}[ht!]
    \begin{center}
        \includegraphics[height=5cm, width=0.85\linewidth]{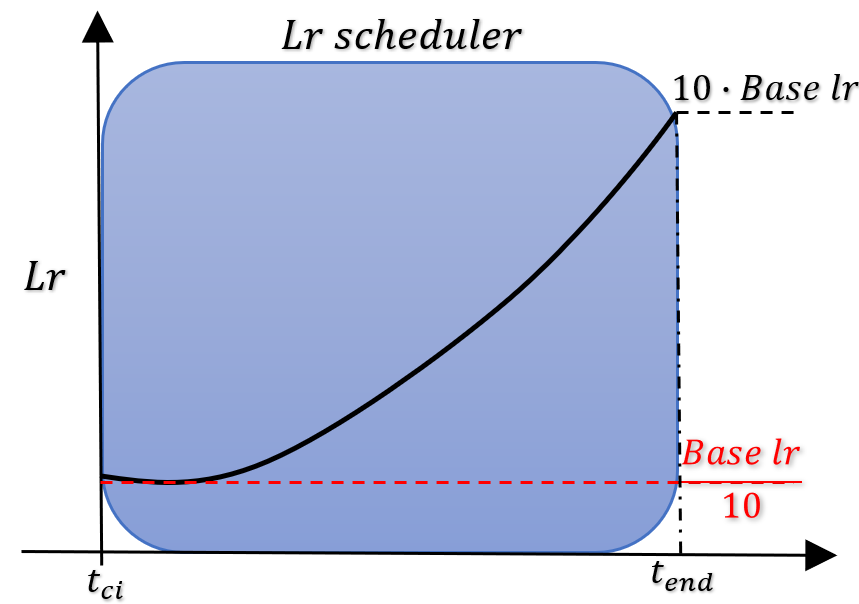 }
    \end{center}  
        \caption{The lr scheduler used in SDAT. $t_{c_i}$ and $t_{end}$ - denotes the starting and ending time index respectively for training over sub-dataset $c_i$.}
	\label{S:LR_SCHEDULER}     
\end{figure}   

\subsection{Models Architecture}
\label{S:model_arch}
In the following we provide a more detailed explanation of the implemented architectures used in the experiments. \\
\textbf{CNN- architecture:}
In the experiments section we provided a range of CNN networks with a varying number of parameters, each architecture consisted of two modules with three Inverted Linear bottlenecks (ILB)\cite{sandler2018mobilenetv2}. By adjusting ILB's "Expansion Factor" hyper parameter, we obtain networks with different number of parameters. The first module operates on the input and produces 12 output channels. Subsequently a pixel shuffle layer transform the output into 3 channels with increased spatial resolution. Then, the second module receives the 3 output channels to produce the final result. \\ 
\textbf{GRL variants architecture:}
We used the GRL-S variant, this architecture receives an RGB image as input, produced by a Matlab demosaic algorithm. As a results the GRL-S model focuses on artifacts removal solution. In order to match our training protocol to be consistent with the other trained networks, as to provide the network a Bayer image as input, we replaced the initial Matlab demosaic with our CNN 16K parameters variant.
\subsection{Qualtitative results}
The following contains supplementary qualitative examples that illustrate the effectiveness of our approach. We compare the outcomes of our SDAT against EDT method.\label{sub:Visual results}\\  
\textbf{EDT in compare to SDAT:} 
We demonstrate a qualitative evaluation  using a 16K parameters model over chosen sub-datasets. We compare between the obtained results using EDT to our SDAT. See Figures \ref{fig:edges} to \ref{fig:zipper}.

\begin{figure*}[ht!]
    \begin{center}
        \includegraphics[height=10cm, width=0.85\linewidth]{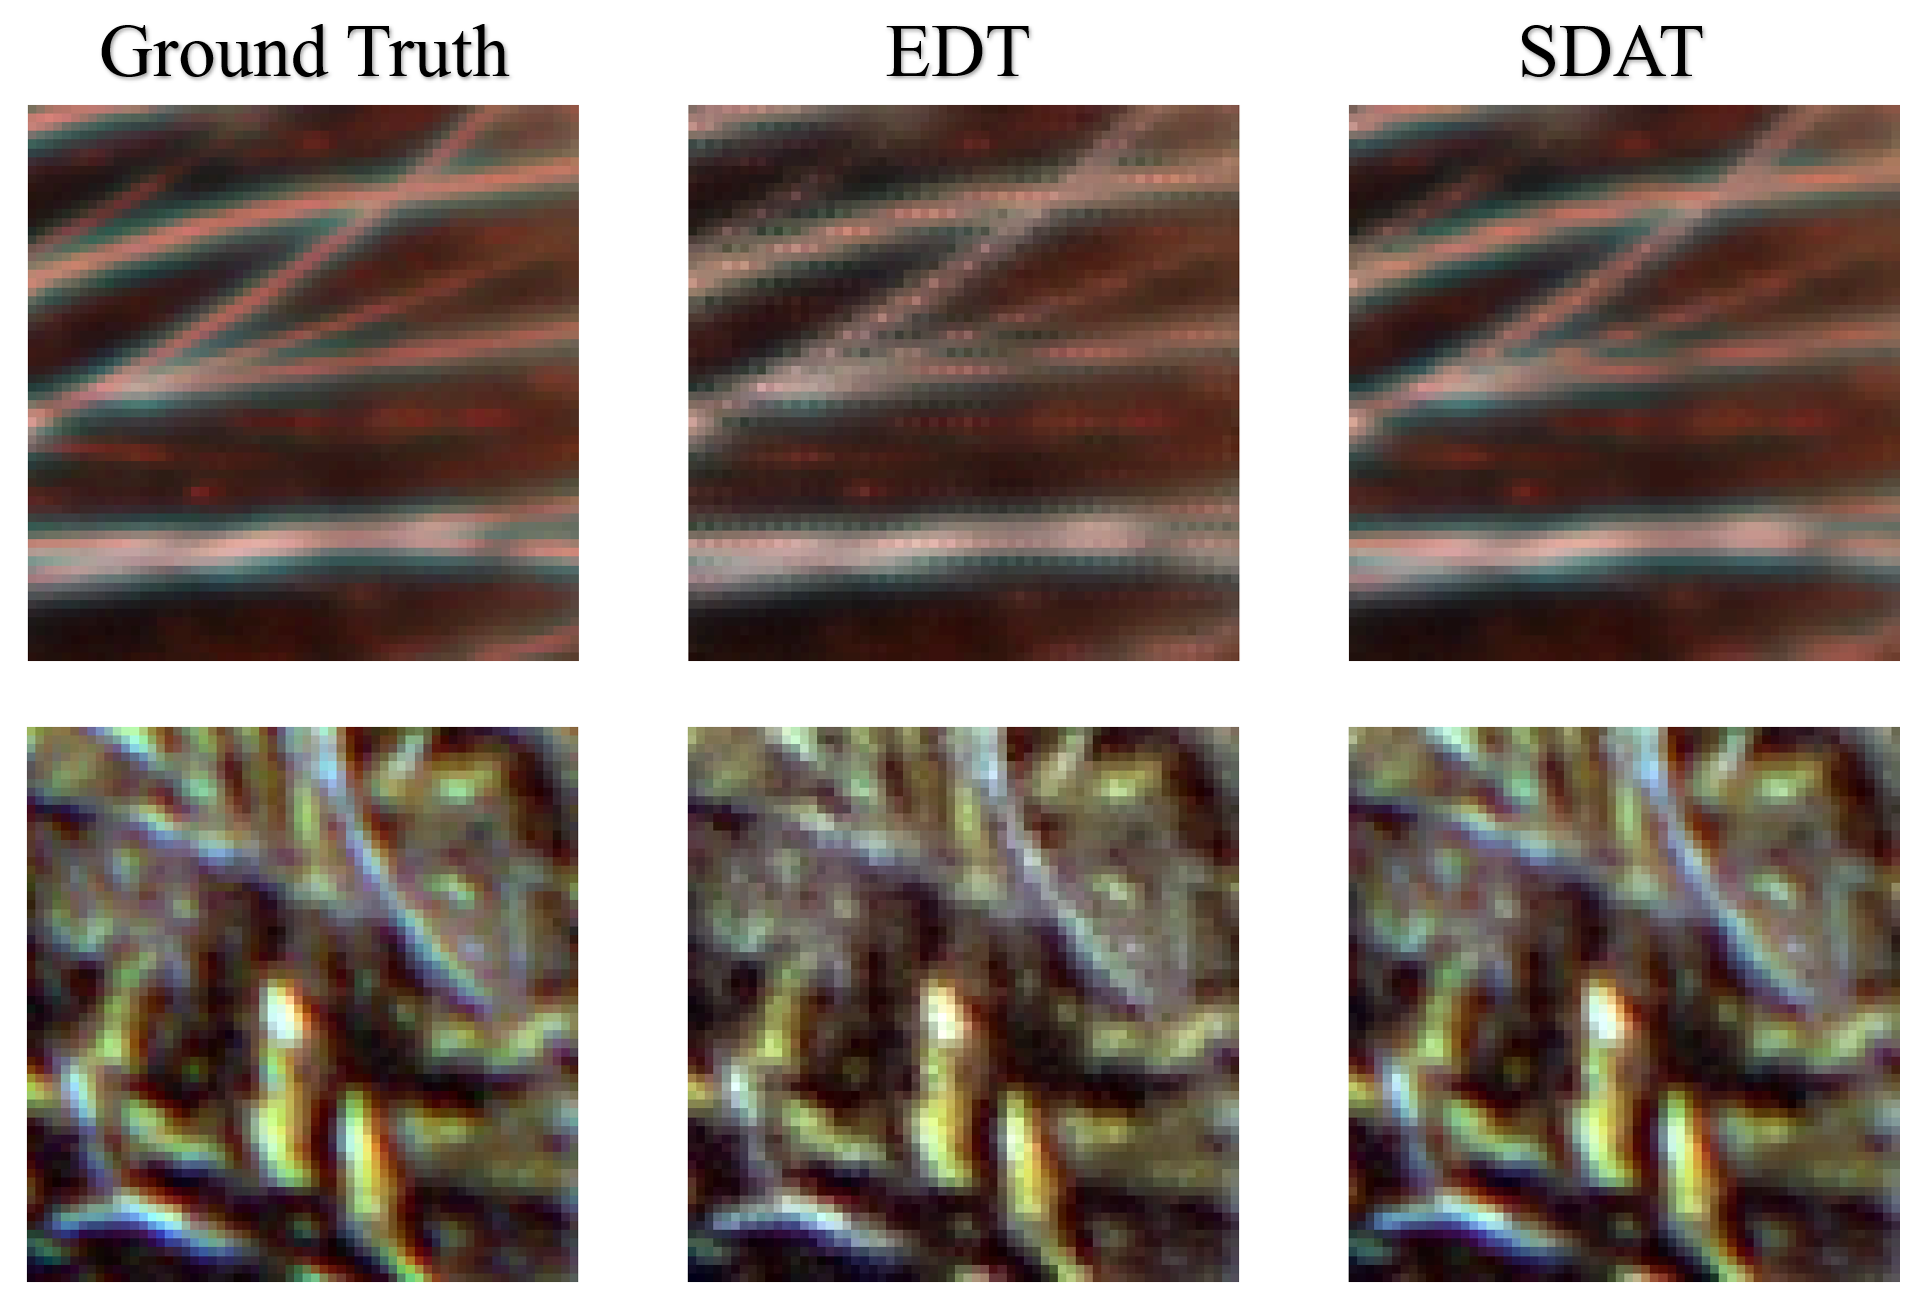 }
    \end{center}  
        \caption{Results for the 16k CNN, using two training methods - EDT and SDAT over sub-dataset obtained by edge metric.}
	\label{fig:edges}   
\end{figure*}            

\begin{figure*}[ht!]
    \begin{center}
        \includegraphics[height=10cm, width=0.85\linewidth]{S_L1_METRIC.png }
    \end{center}  
        \caption{Results for the 16k CNN, using two training methods - EDT and SDAT over sub-dataset obtained by L1 metric.}
	\label{fig:l1}   
\end{figure*} 
   
\begin{figure*}[ht!]
    \begin{center}
        \includegraphics[height=10cm, width=0.85\linewidth]{S_GRID_METRIC.png }
    \end{center}  
        \caption{Results for the 16k CNN, using two training methods - EDT and SDAT over sub-dataset obtained by Grids metric.}
	\label{fig:grids}   
\end{figure*} 

\begin{figure*}[ht!]
    \begin{center}
        \includegraphics[height=10cm, width=0.85\linewidth]{S_PERCEP_METRIC.png }
    \end{center}  
        \caption{Results for the 16k CNN, using two training methods - EDT and SDAT over sub-dataset obtained by Perceptual metric.}
	\label{fig:perceptual}     
\end{figure*} 

\begin{figure*}[ht!]
    \begin{center}
        \includegraphics[height=10cm, width=0.85\linewidth]{S_ZIPPER_METRIC.png}
    \end{center}  
        \caption{Results for the 16k CNN, using two training methods - EDT and SDAT over sub-dataset obtained by Zipper metric.} 
	\label{fig:zipper}   
\end{figure*}  

\begin{figure*}[h!]
    \begin{center}
        \includegraphics[height=9cm, width=1\linewidth]{kodak_1.png}
    \end{center}    
        \caption{Qualitative result using three models with increasing number of parameters: 16K, 84k and 900k over image 1 in Kodak dataset  \cite{li2008image} .}
	\label{fig:kodak_1}   
\end{figure*}

\begin{figure*}[ht!]
    \begin{center}
        \includegraphics[height=9.5cm, width=1.05\linewidth]{Kodak19.png}
    \end{center}  
        \caption{Qualitative result using three models with increasing number of parameters: 16K, 84k and 900k  over image 19 in Kodak dataset \cite{li2008image} .  }
	\label{fig:kodak_19}   
\end{figure*}   

\iffalse

\begin{figure*}[ht!]
  \centering
  \subfloat[] {\label{fig:subfig1}
    \includegraphics[height=10cm, width=1.05\linewidth]{urban_86.png}
    }
    \hspace{0.4\linewidth}
   \subfloat[] {\label{fig:subfig2}
    \includegraphics[height=10cm, width=1.05\linewidth]{urban_28.png}
  }
  \caption{Qualitative comparison of our method compared to other top methods RNAN and RSTCANet. The RNAN model has 9M parameters, while RSTCANet-B , RSTCANet-S and RSTCANET-L have 0.9M , 3.1M and  7.1M respectively.}
  \label{fig:merged}
\end{figure*}
\fi

\textbf{Qualitative results over different models:}
In the following, we present the outcomes of our training method utilizing three models with varying parameter counts, namely 16k, 84k, and 900k parameters. To construct the 16k and 84k parameter models, we utilized our CNN variants as explained in \cref{S:model_arch}, while for the 900k parameter model, we implemented the RSTCANetB architecture \cite{xing2022residual}. We demonstrated over chosen examples from Kodak dataset \cite{li2008image}. See in Figures \ref{fig:kodak_1} and \ref{fig:kodak_19}.
\iffalse
\subsection{Our method compare to top demosaicing solutions}
Qualitative comparison of our method to other leading demosaicing methods, RNAN \cite{zhang2019residual} and RSTCANet over chosen images from Urban100 \cite{huang2015single}. RNAN comprises 9M parameters,  RSTCANet consists of three different model sizes  B, S, and L  with 0.9M, 3.1M, and 7.1M parameters, respectively. We use our suggested training scheme to train the B model.  Our results, as shown in \Cref{fig:merged}, demonstrate that our method outperforms the RSTCANet-B method, which has the same architecture, and also outperforms RSTCANet-S and RNAN, despite having significantly fewer parameters. When compared to RSTCANet-L, our RSTCANet-B produces similar results, with a slight advantage towards RSTCANet-L in some cases.
\fi
%\input{references.tex}
